# Supplementary material for: Suppression of Density Fluctuations in a Quantum Degenerate Fermi Gas
Source: arXiv:1005.1309 source file (2010-05-24)
Supplement: Supplementary file 1 [file supplement.pdf]

# Suppression of Density Fluctuations in a Quantum Degenerate Fermi Gas: Supplementary Information

## EXPERIMENTAL DETAILS

To accurately measure the atom number variance it is necessary to eliminate patterns in the absorption images whose fluctuations increase the observed noise. Weak reflections of the probe beam from the walls of the glass cell and from optical elements in the imaging system can interfere with the probe beam itself, leading to spatial fluctuations in its intensity profile. To reduce interference fringes and ensure uniform illumination, the central area of the probe beam is imaged onto the sample through a 2 mm aperture. Even though the residual fringes are small, there are two significant effects of inhomogeneous illumination which must be addressed.

First, if the time elapsed between the image with atoms and the reference image without atoms is too large, mechanical vibrations of the optics will cause the intensity profile of the probe to change between the two images, creating artifacts in the absorption image. To reduce this effect, we operate our CCD in fast kinetics mode, with a time interval $\approx 500\mu s$ between exposures. Since there is no longer enough time for the atoms to exit the frame between images, before taking the reference image we optically pump the atoms from the $|1\rangle$ state to the $|6\rangle$ state, and from the $|2\rangle$ state to the $|5\rangle$ state ($|1\rangle$ refers to the lowest hyperfine state, etc.), by exciting them to the $m_J = 1/2$ excited state manifold. At the magnetic fields used in the experiment, these levels are separated in frequency from the $|2\rangle$ state used for imaging by $\approx 2$ GHz and contribute negligibly to resonant imaging.

Second, if the average probe intensity is too high, the atoms subjected to higher intensities will have a lower effective cross-section, and so any spatial fluctuations in the beam intensity will be 'imprinted' onto the absorption images. As a result, in our experiment we use a probe beam with maximum intensity of 0.12 of the saturation intensity $I_{sat}$=2.54 mW/cm$^2$, where these effects are relatively small. The variation of optical density with intensity is shown in Fig. 1.

Additionally, the exposure time must be kept very short to prevent the atoms from moving between pixels during the exposure. The expected motion of atoms during the 4 $\mu$s exposure is on the order of 1 $\mu$m, much smaller than the effective pixel size.

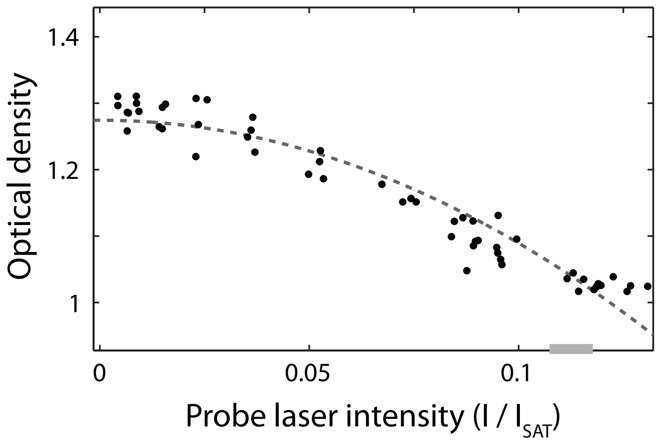


FIG. 1: Determination of the absorption cross section. The observed optical density decreases with increasing probe light intensity. The line is a quadratic fit to the data. The reduction of the cross section is mainly due to the Doppler effect caused by acceleration of the atoms by radiation pressure; a smaller reduction results from the partial saturation of the optical transition. At the probe light intensity chosen in this study (shaded bar), the number of photons absorbed per atoms is about 6. The decrease of the cross section is slightly larger than that predicted by simple models.

## NOISE DETERMINATION

In this experiment the local atom number variance is determined by comparing the measured number of atoms in the same bin across a series of images. To do this, we must first eliminate the effect of fluctuations in the total atom number between experimental cycles. Initially, we select the 85 images used in the analysis from a larger group of $\approx 150$ images, using an automated procedure to choose the images whose total atom numbers are closest to the center of the distribution. A very small number of images ($< 1\%$) are manually excluded because of obvious artifacts in the frame due to dust particles or other large perturbations. Then, we subtract a fitted profile from each OD image before computing the variance. Initially we subtracted a fitted 2D Thomas-Fermi profile, but we replaced this with a Gaussian fit which had an insignificant effect on the variances, while taking considerably less computation time.

We then compute the variance in optical density at each position. That variance has contributions from photon and atom shot noise, given by the following formula:

$$(\Delta(OD))^2 = \frac{1}{\langle N_1\rangle} + \frac{1}{\langle N_2\rangle} + \frac{\sigma^2}{A^2}(\Delta N_{atom})^2 \qquad (1)$$

This equation holds bin by bin: $N_1$ is the average number of photons measured in a given bin position for the image with atoms, and $N_2$ is the average number of photons measured in that bin for the reference image. $(\Delta N_{atom})^2$ is the variance in atom number for that bin, $\sigma$ is the

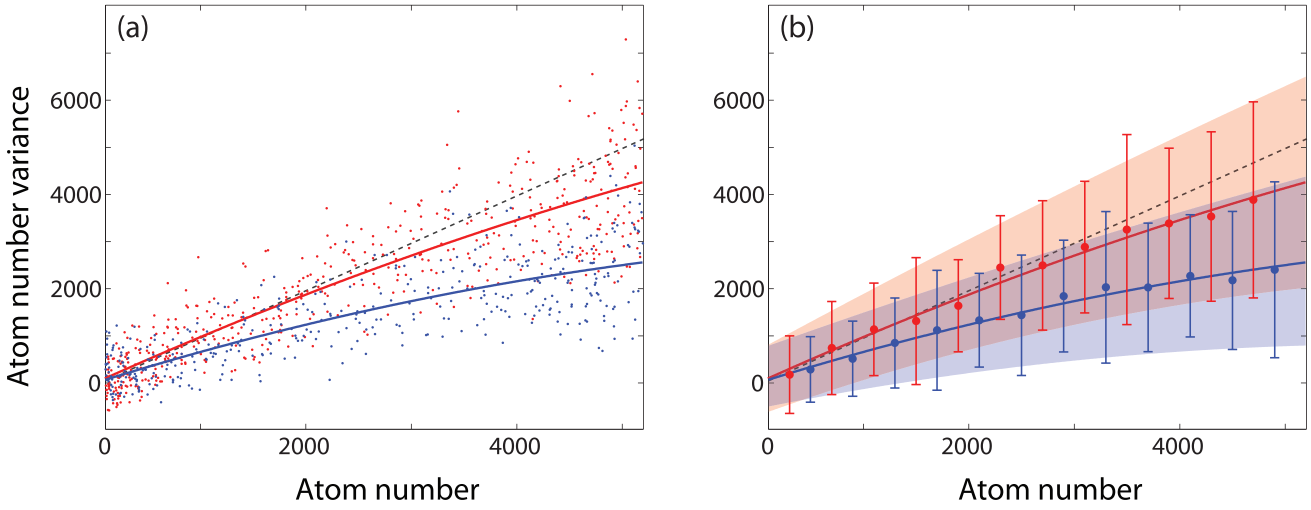


FIG. 2: Atom number variance vs. atom number. (a) Data for all of the resolution elements is plotted. Red points are from the hot cloud at $T/T_F = 0.6$, blue points from the cold cloud at $T/T_F = 0.21$. There is significant scatter in the variance data, and there are many "cold" pixels which actually have higher variance than their corresponding "hot" pixel. (b) The red and blue shaded regions indicate the expected $2\sigma$ scatter in sample variance that is expected due to atom and photon counting statistics. The large circles are variance data averaged over pixels with similar atom number for hot (red) and cold (blue) cloud. The bars show the measured $2\sigma$ scatter of the data points. The measured scatter agrees very well with the expected scatter, indicating that the scatter of the data is fully accounted for by counting statistics. Negative values of the observed atom number variance result from the subtraction of photon shot noise.

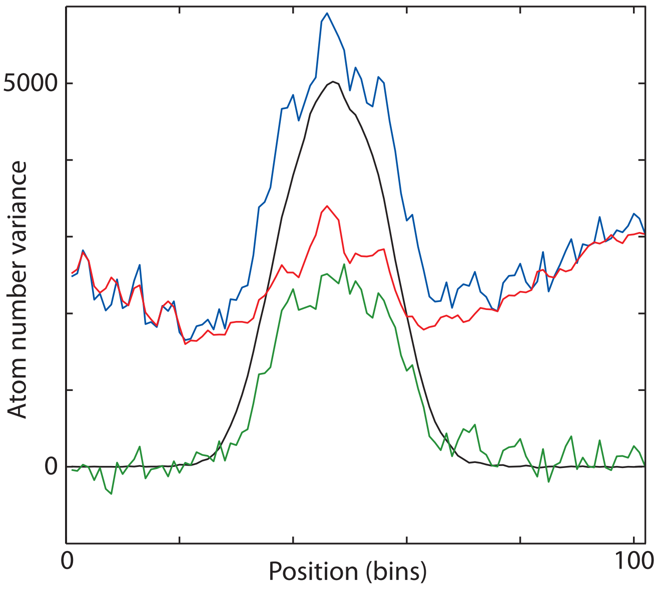


FIG. 3: Determination of profiles of the atom number variance for a cold cloud. For each bin, the total photon count is determined, and its contribution (red) to the total variance of the optical density (blue) is subtracted. The obtained atom number variance (green) is compared to the average atom number (black). The displayed trace reveals 50% noise suppression in the center of the cloud. The apparently high suppression of atom variation in the wings is a statistical fluctuation. Fig. 2 shows that the suppression is monotonic in atomic density.

absorption cross section, and $A$ is the effective bin area. The atom number variance is isolated by calculating the first two photon shot noise terms and subtracting them. The analysis used in the paper also subtracts contributions from detector read noise and photon shot noise in the dark field, but these are fairly small contributions.

The determination of $N_1$ and $N_2$ depends on the CCD gain, which is measured to be 1.18 (counts/electron) from $\approx 240$ pairs of images without atoms, employing the assumption that the detector statistics are Poissonian. After the subtraction of photon shot noise (and technical noise), the remaining variance in optical density is due to the atom number variance. Fig. 3 shows the contributions of photon and atom number variance to the overall noise in optical density.

The large scatter of the measured atom number variance, as depicted in Fig. 2, is not primarily due to technical noise, but instead a statistical property of the sampling distribution of the variance. The shaded areas are derived from theoretical values for the variance of the sample variance. This is given by

$$\mathrm{Var}(\mathrm{Var}(N)) = \frac{(m-1)^2}{m^3}\mu_4 - \frac{(m-1)(m-3)}{m^3}\mu_2 \quad (2)$$

where m is the number of observations in each sample. The moments $\mu_2$ and $\mu_4$ are the central moments of the population distribution. For a Poisson distribution, $\mu_2 = \langle N \rangle^3$ and $\mu_4 = \langle N \rangle(1 + 3\langle N \rangle)$, and for $m, \langle N \rangle \gg 1$, this expression reduces to $2\langle N \rangle^2/m$. Fig. 2b shows the

comparison between the expected and measured variance in the sample variance.

## IMAGING SYSTEM CHARACTERIZATION

The blurring of adjacent pixels due to finite optical resolution effectively decreases the measured atom number variance. This effect is avoided by binning the data using a sufficiently large bin size (Fig. 5). In our experiment, this bin size is determined by the extension of the cloud along the optical axis, which is much larger than the depth of focus of the diffraction limit of the lens system.

Atom noise allows us to characterize the transfer function of our imaging system. Fig. 4 shows the average power spectrum (modulus squared of the spatial Fourier transform) of the optical density images. Because the Fourier transform of uncorrelated fluctuations is flat, the deviation from flatness of the density noise corresponds to blurring induced by the lens, barring the central peak corresponding to the shape of the cloud. For wavevectors $q$ much larger than the resolution limit of the detection scheme, the atom number fluctuations are no longer imaged, and the power spectrum is the photon shot noise. For our experiment this happens for $q < q_F$. Comparison of the power spectra for the cold and the hot cloud shows, at small values of $q$, a 50% suppression, consistent with the results obtained using spatial bins. If the imaging system still had contrast at $q > 2q_F$, we would expect the ratio of the power spectra to approach unity, since momentum transfer $q > 2q_F$ to a Fermi cloud has negligible Pauli suppression.

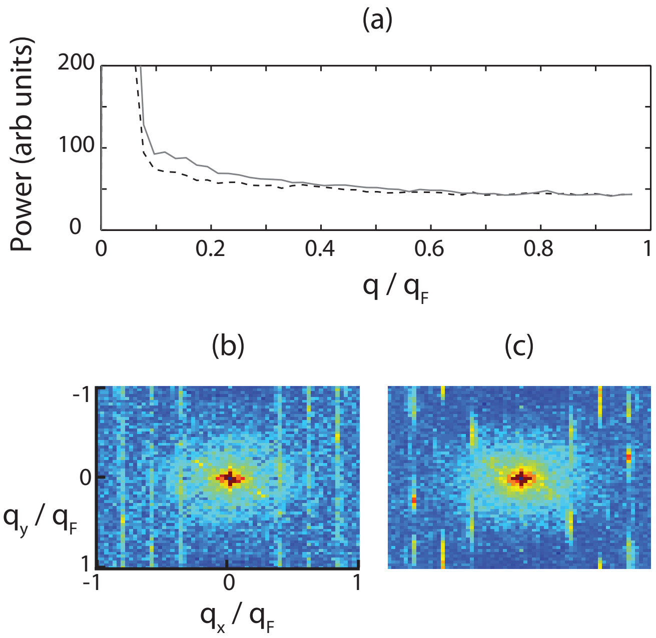


FIG. 4: (a) Radially averaged power spectra of optical density images for hot (solid line) and cold (dashed line) samples (b) Power spectrum of cold sample (arbitrary units) (c) Power spectrum of hot sample (arbitrary units). A constant offset is added to the power spectrum for the hot sample to equalize the levels of photon shot noise.

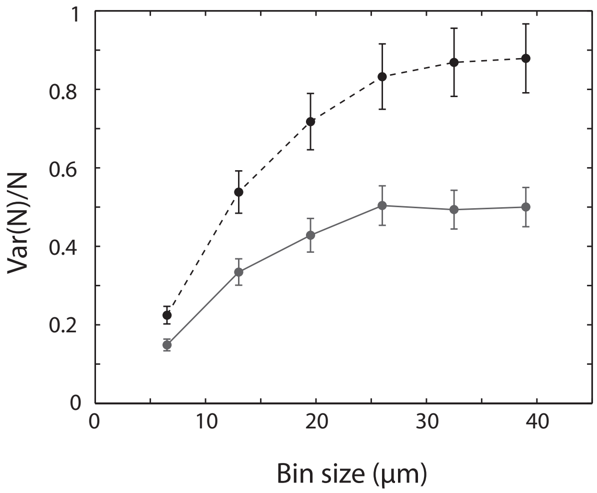


FIG. 5: Observed atom number variance versus bin size for heated (dashed line) and cold (solid line) samples, normalized to 1 for Poissonian statistics. A plateau is reached when the blurring of the bins due to finite optical resolution is negligible.
